# Supplementary material for: Amalur: Data Integration Meets Machine Learning
Source: arXiv:2205.09681 source file (2023-03-01)
Supplement: Supplementary file 1 [file 8_appendix.tex]

\cleardoublepage
\appendix
Generation of mapping matrices $M_1$ and $M_2$ from the schema mapping $m$ is straightforward, as shown in Alg.~\ref{alg:MMGen}. 
We explain Alg.~\ref{alg:MMGen} with the following example.
\begin{exmp} 
	\label{exmp:mm_full}
% Fig.~\ref{fig:allMs} b marks the column numbers of the mapped attributes (from their own matrices) in the schema mapping $m$. 
We continue with the running example. 
The inputs of Alg.~\ref{alg:MMGen} include $\mathcal{M} =\{m_1, m_2,m_3 \}$,  $\mathbf{S}=\{S_1, S_2\}$ and $T$.
Fig.~\ref{fig:allMs}a shows the output $\mathbf{M}=\{M_1, M_2\}$.
$T$  has 4 columns. 
The  numbers of mapped columns in $S_1$, $S_2$ are 3 and 3 respectively.   
Following the above definition, by line \ref{alg:MMGen:zeroM} of Alg.~\ref{alg:MMGen} we create two zero matrices: $M_1$ with the shape $4 \times 3$ and $M_2$ with the shape $4 \times 3$. 
Via line \ref{alg:MMGen:indexCol} and  \ref{alg:MMGen:defBeg}-\ref{alg:MMGen:map} the column matching information is added to $M_1$ and $M_2$ following the above definition. 
For instance, from $m_1$ we have $S_1.s$ (column ID: 0) mapped to   $T.s$ (column ID: 0), thus, $M_1[0,0] =1$. 
\end{exmp}
\setlength{\textfloatsep}{0pt} 
\begin{algorithm}[tb]
	\caption{MappingMatrixGen}
	\label{alg:MMGen}	
	%	\setstretch{0.85}
	\DontPrintSemicolon
	\KwIn{Schema mappings $\mathcal{M}$, source schemas $\mathbf{S}$, target    schema $T$
		\\{\bf Output}: Mapping matrices $\mathbf{M}$}
	\SetKwBlock{Begin}{function}{end function}

	\bf Initialization: $\mathbf{M} \gets \emptyset, m, n \gets 0$
	
	$n\gets countColNum(T)$\tcp{number of columns in $T$}\label{alg:MMGen:dimT}
	
	\ForEach{$S_k \in S$}{
	  $\mathbf{J} \gets getMappedColIDs(S_k, \mathcal{M})$ \label{alg:MMGen:indexCol}
	  
	  	  $m \gets count(\mathbf{J})$ \tcp{number of mapped columns in $S_k$  } \label{alg:MMGen:dim}
	  	  
	  	  $M_k \gets createInitialMatrix(n,m)$\label{alg:MMGen:zeroM}

	  \ForEach{$j \in \mathbf{J}$}{ \label{alg:MMGen:defBeg}
	  \tcp{$ j^{th}\ col\  of\  S_k\  is\  mapped\  to\  the\    i^{th}\ col\  of\  T$}
	      $i \gets getMappedTColIndex(j, \mathcal{M})$ 
          
          $M_k[i,j] \gets 1$ \label{alg:MMGen:map}
	       
	  }
	  
	  $add \ M_k \ to\ M$
	  
}
	\Return $\mathbf{M}$
\end{algorithm}

To generate compressed mapping matrices, the vector $CM_k[i]$ is initialized with values of $-1$ in line  \ref{alg:MMGen:zeroM}, and  line~\ref{alg:MMGen:map} of Alg.~\ref{alg:MMGen} needs to be changed to 	$CM_k[i] \leftarrow j$. 

\subsection{Indicator matrix generation}

\setlength{\textfloatsep}{0pt} 
\begin{algorithm}[tb]
% \asterios{readers can come up with making a nicer representation of a sparse matrix without this pseudocode, right? If we show them the original matrix and its compressed version? Also, this matrix being conpressed is an optimization and does not affect at all the findings of this paper, it could sdafely be left to its sparse version and we could save lost, and lots of space to talk about the actual vision, insread of how to compress a matrix (which I would include in a research paper, but not here).}
	\caption{CompressedIndicatorMatrixGen}
	\label{alg:IMGen}	
	%	\setstretch{0.85}
	\DontPrintSemicolon
	\KwIn{Row matching $\mathbf{N}$, schema mappings $\mathcal{M}$, source tables $\mathbf{D}$  
		\\{\bf Output}: Compressed Indicator matrices $\mathbf{CI}$}
	\SetKwBlock{Begin}{function}{end function}
	
	\bf Initialization: $\mathbf{CI} \gets \emptyset, l_T \gets 0, r \gets 0$
	
		\ForEach{non-singleton- LHS mapping $m \in \mathcal{M}$\label{alg:IMGen:mapping:begin}}
		{   
		    \tcp{initial rows are merged rows from multiple sources}
            $l_T, r \gets countMergedRows(m, \mathbf{N})$\label{alg:IMGen:mapping:end}
            
        %   $l_T \gets r$ \label{alg:IMGen:mapping:end}
		}
		
		\ForEach{$source\ table\ D_k \in \mathbf{D} $\label{alg:IMGen:eachTable:begin}}
		{
		    $CI_k \gets createDynamicRowMatrix(l_T)$
		    
		    $CI_k \gets fillMergedRowID(\mathbf{N}, r, CI_k)$ \label{alg:IMGen:mergedRow}
		  %  \tcp{fill in the first r elements of $CI_k$}
		    
		    \If{singleton- LHS mapping $m_k \in \mathcal{M}$}{
 
            $CI_k, l_T \gets addRestRowsID(D_k, CI_k, l_T)$ \tcp{update $CI_k$, $l_T$}
            \label{alg:IMGen:restRow}
            }
            $add\ CI_k \ to \ \mathbf{CI}$\label{alg:IMGen:eachTable:end}

		}

	$\mathbf{CI} \gets fillNullValues (\mathbf{CI})$\tcp{unify vector lengths} \label{alg:IMGen:fillNull}
	
	\Return $\mathbf{CI}$
\end{algorithm}

\para{Matrix generation}  Alg.~\ref{alg:IMGen} 
  outlines  our approach to generate compressed indicator matrices. 
The main intuition is to add IDs of  overlapped rows first, then  sequentially add the rest  row IDs of each source table. Different from  mapping matrix generation in Alg.~\ref{alg:MMGen}, we do not prefix 
the size of a compressed indicator matrix but dynamically obtain it during matrix generation.
% Before illustrating Alg.~\ref{alg:IMGen} with  Example~\ref{exmp:cimGen}, we first explain its three inputs.

\para{Algorithm inputs} 
The first inputs are row matching pairs $N$ between source tables. For example, in Fig.~\ref{fig:allMs}b, $N=\{[D_1[3], D_2[2]]\}$. These two rows are matched and both contribute to the generation of $T[0]$. If a row of $T$ is from more than one source, we call it a \emph{merged row}, e.g.,  $T[0]$.
% \asterios{the LSH should be LHS? LSH reminds me of locality sensitive hashing and messes up with my brain. Same for the algorithm 2.}
Second, given a tgd in $\mathcal{M}$, if in the left-hand-side ( LHS) of the implication ($\rightarrow$) there are  relational atoms from multiple sources, we call it  a   \emph{non-singleton- LHS} tgd, which indicates the chosen sources contributing to the merged rows of $T$.
% that the overlapped rows from different sources contribute to rows of $T$, while  singleton- LHS tgds specify that  rows from the single source will also contribute to $T$.
For example, in Fig.~\ref{fig:motiv}c $m_1$ is a non-singleton- LHS tgd while $m_2$ and $m_3$ are singleton- LHS tgds. 
The third inputs of Alg.~\ref{alg:IMGen} are the processed  source tables $\mathbf{D}$ as shown in Fig.~\ref{fig:allMs}b.
Notably, for the downstream ML algorithms, not all but only partial data of an original source table will  participate the computation as features or labels. 
% from the source tables only the data of mapped columns , i.e., . 
Thus, we transform the original tables $S_1$ and $S_2$ in Fig.~\ref{fig:motiv}a-b to their matrix forms $D_1$ and $D_2$  in Fig.~\ref{fig:allMs}b, which only include the mapped columns. 
The transformation also includes data   preprocessing operations, e.g.,
% dropping useless columns (e.g., $S_2.d$),
one-hot encoding (\textit{female $\rightarrow$ 0}, \textit{male  $\rightarrow$ 1}).

\begin{exmp} 
	\label{exmp:cimGen}
\vspace{-0.1cm}	
For the running example, 
  Alg.~\ref{alg:IMGen} outputs $\mathbf{CI}= \{CI_1,CI_2\}$.
% Intuitively, from $CI_1$, $CI_2$ in Fig.~\ref{fig:allMs}b we can see that the first four rows of $T$ are from $D_1$, while the first and last two rows of $T$ are from $D_2$.
Alg.~\ref{alg:IMGen} has four steps. 
(i) In line \ref{alg:IMGen:mapping:begin}-\ref{alg:IMGen:mapping:end}, we process  $m_1$, since among three tgds  it is the only non-singleton- LHS tgd. With the join relationship indicated by $m_1$, the function \textit{countMergedRows} examines the row matching pairs of $D_1$ and $D_2$ in $N$, and counts the number of merged rows, 
% . Since rows $D_1[3]$ and $D_1[2]$ are matched, 
$l_T=r=1$. 
% c shows the compressed indicator matrices $CI_1$ and 	$CI_2$ following Definition~\ref{def:cim}. 
% Next, we show how they are generated. 
(ii) Next, via line \ref{alg:IMGen:eachTable:begin}-\ref{alg:IMGen:eachTable:end}, 
sequentially we process $D_1$ and $D_2$ and dynamically generate their compressed indicator matrices.
With line~\ref{alg:IMGen:mergedRow} we tackle
% row matching of 
merged rows first. 
% That is, 
Given a merged row, e.g., $T[0]$, the corresponding row IDs in the source tables $\mathbf{D}$ are added to $CI_k$, e.g., $CI_1 = [0]$, $CI_2 = [2]$.
(iii) Then we add  the rest rows of each source table. 
For instance, after processing $D_1$, $CI_1 = [3, 0, 1, 2]$, $l_T=4$.
For $D_2$, via line~\ref{alg:IMGen:restRow} we   extend $CI_2$ to the same length of $CI_1$ by filling the value  of $-1$,
% from position $r$ to  $l_T-1$;
then add  the rest non-merged rows from $D_2$ and update  $l_T$.
% starting from the location of $l_T$, 
$CI_2 = [2, -1, -1, -1, 0, 1]$ and $l_T = 6$. 
(iv) Finally, via line~\ref{alg:IMGen:fillNull} each $CI_k$ is adjusted to the final vector length $l_T$ by filling the empty elements with  $-1$, e.g., $CI_1$ is adapted to $[3, 0, 1, 2, -1, -1]$. 

\para{Algorithm extension} In the running example we only showed the simple case that rows are matched in pairs with equal values. It can be extended to more general data matching results. That is, similar records from different sources are group as clusters \cite{10.1145/775047.775116}, or  values are matched   semantically or with specific rules \cite{he2015sema}, e.g., sex values of female/male and $f/m$. The key to extend Alg.~\ref{alg:IMGen} is to redefine   $N$ and related functions according to data matching inputs.   

\vspace{-0.2cm}
\end{exmp} 

\para{Feasibility of indicator matrix construction} In the running example we only showed the simple case where rows are matched in pairs with equal values. 
Such linkages of rows can be the results of  entity linkage and disambiguation \cite{brizan2006survey}, which are intensively studied  fields with matured tools. It is an interesting future direction to extend
the definition of   (compressed) indicator matrix   according to more general data matching results. That is, similar records from different sources are group as clusters \cite{10.1145/775047.775116}, or  values are matched   semantically or with specific rules \cite{he2015sema}, e.g.,   $female/male \leftrightarrow   f/m$. 

\para{Redundancy matrix generation} For brevity we discuss the simple case of two source tables, which can be  extended to multiple sources. We assume that to construct $T$ the base table is $D_b$ and overlapped values in the current table $D_k$ is redundant. 
Given mapping matrices $M_b, \ M_k$ and indicator matrices $I_b, \ I_k$, we can transform them into $R_k$ with row summarization ($rowSums(\cdot)$), element-wise multiplication ($\circ$)
%Hadamard product   
outer product ($\otimes $), and logical negation ($\neg$ ). 
\vspace{-0.2cm}
\begin{align*}
	R_k = 
\neg((rowSums(I_b)\circ & rowSums(I_k)) \otimes \\ &(rowSums(M_b)\circ rowSums(M_k)))  
\vspace{-0.2cm}
\end{align*}
